# Supplementary material for: A new look on the two-dimensional Ising model: thermal artificial spins
Source: arXiv:1507.01126 source file (2015-07-04)
Supplement: Supplementary file 1 [file Supplementary_material_Arx.pdf]

# A new look on the two-dimensional Ising model: thermal artificial spins

## Supplementary material

Unnar B. Arnalds, Jonathan Chico, Henry Stopfel, Vassilios Kapaklis, Oliver Bärenbold,
Marc A. Verschuuren, Ulrike Wolff, Volker Neu, Anders Bergman, and Björgvin Hjörvarsson
(Dated: July 2, 2015)

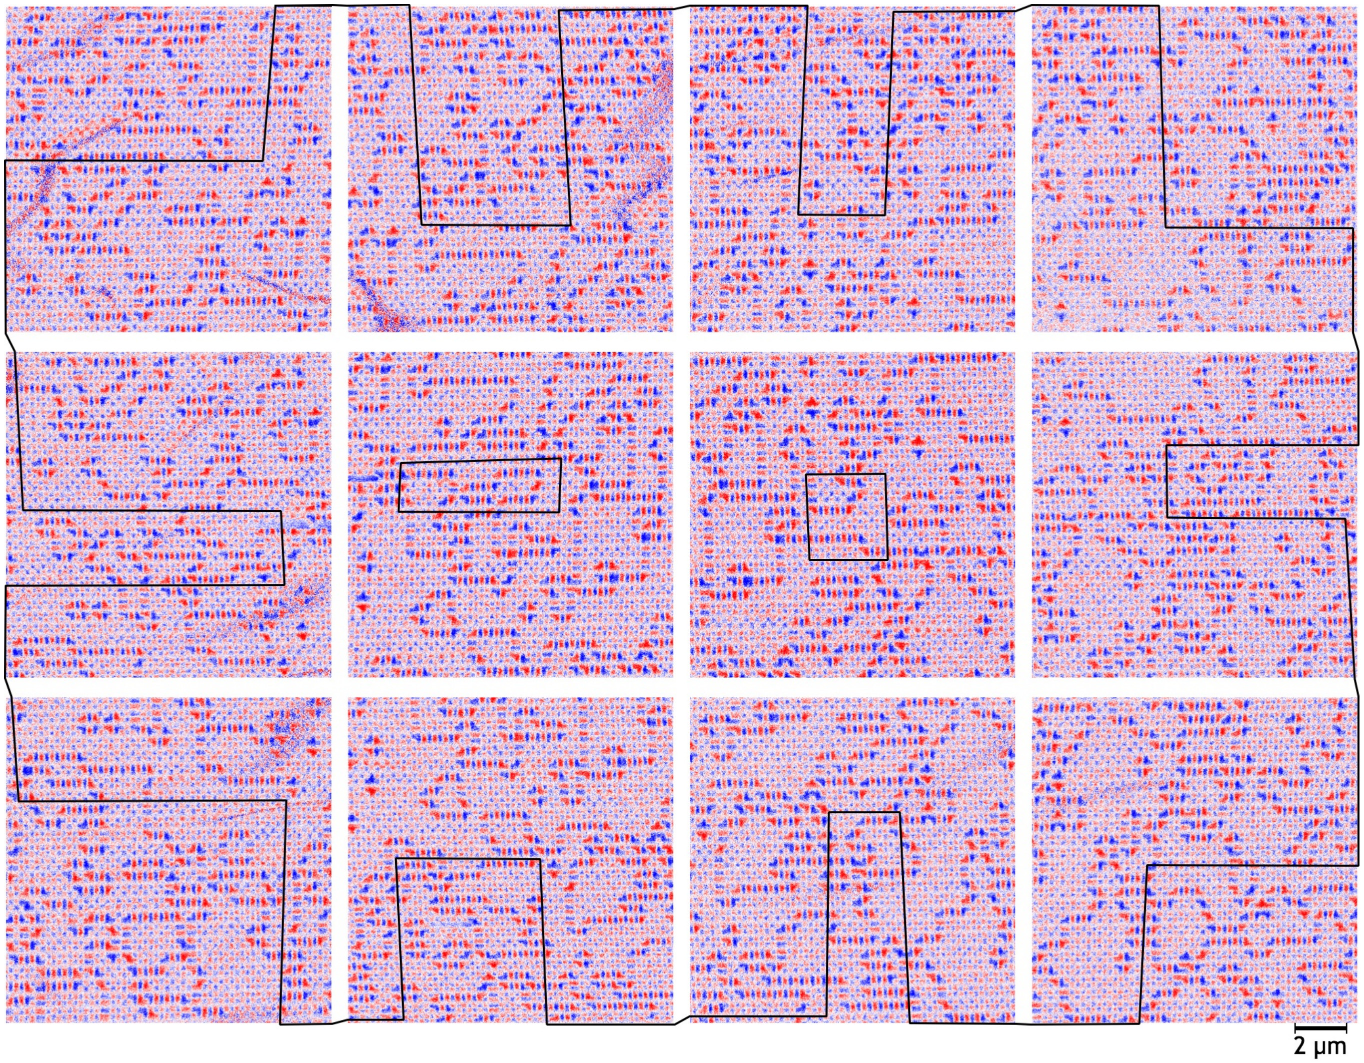


FIG. 1. Magnetic force microscopy (MFM) images. The combined array used for the investigation was created from a set of 12 MFM images (see Methods) with overlapping regions where each image consisted of a $12\times12$ $\mu$m$^2$ scans. The solid black lines reveal the areas which are overlapped between neighboring images. No differences were observed between the overlapping areas indicating that the magnetization direction of the islands was not affected by the stray field of the MFM tip.

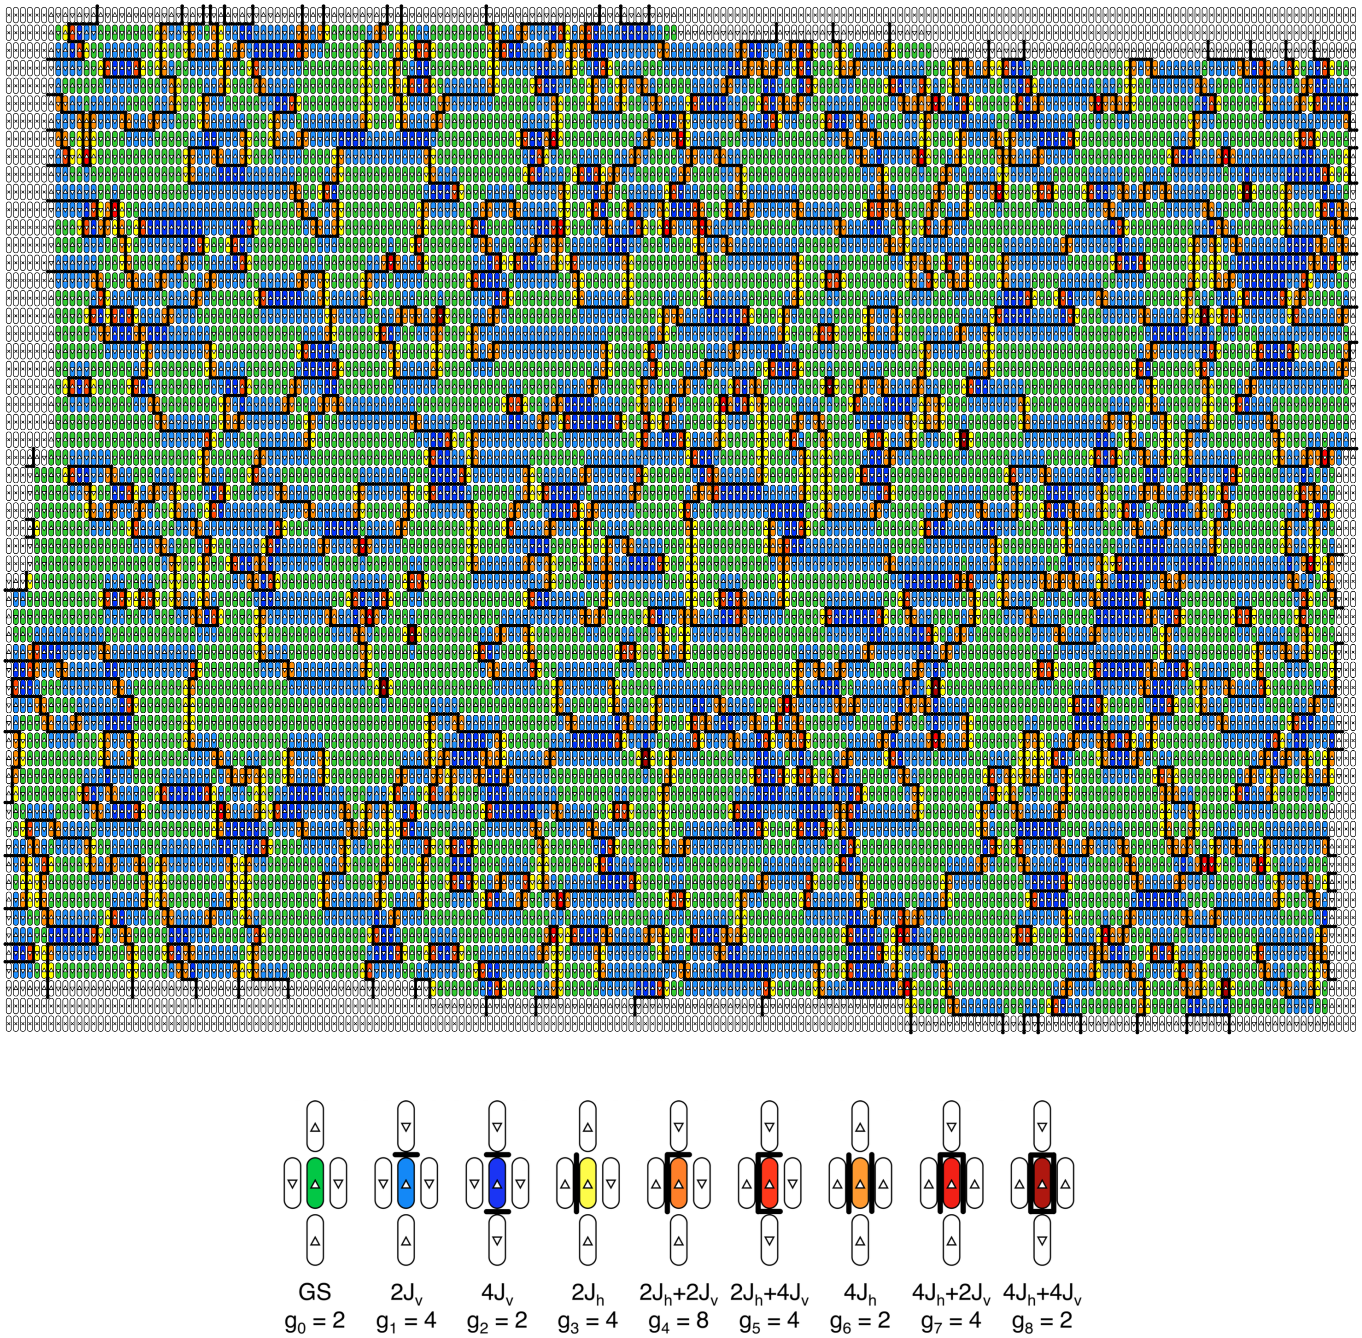


FIG. 2. Array energy state overview. An overview showing the determined magnetizatin direction of all the islands in the array. The lower image shows the colour coding used for labelling the different energy states of the islands assuming a nearest neighbor interaction scheme. A datafile with the determined magnetization directions of the islands for the array is provided as a supplementary file. In the data file islands pointing down are given a value of 0 while islands pointing up are given a value of 1. Due to drift in the MFM imaging the final array of determined islands was not square and therefore islands along the edges of the array with an undetermined magnetization direction were introduced into the datafile with values of 2.
